# Supplementary material for: Paying More Attention to Self-attention: Improving Pre-trained Language Models via Attention Guiding
Source: arXiv:2204.02922 source file (2022-04-06)
Supplement: Supplementary file 1 [file appendix.tex]

\clearpage

\section*{APPENDICES}

We present additional details on our experimental in the appendices below.
We include the source code (Appendix~\ref{app:subsection:code}); the average runtime of each module and detailed information about the parameters (Appendix~\ref{app:section:runtime}); the downloadable links about the used datasets (Appendix~\ref{app:section:dataset});
and ethical considerations
(Appendix~\ref{app:section:ethics}).

\appendix

\section{Code}
\label{app:subsection:code}
Our code is uploaded to \url{https://OpenReview.net} with the paper.
% Our code is available at:  \url{https://github.com/anonymous}.
% \mdr{Give a url for an anonymous repo.}

\section{Runtime and Parameters}
\label{app:section:runtime}
% \mdr{See \url{https://aclrollingreview.org/authorchecklist} under reproducibility, second main bullet.}
% In terms of average runtime, the time cost for our BERT-\ac{MCRF} model is acceptable.
% The time costs for BERT-\ac{MCRF} is 2 hours.
% The run time of BERT-CRF is the same with BERT-\ac{MCRF} and the run-time for BERT is less than 1 hour.
In terms of average runtime, the time cost for all \acp{PLM} with the proposed \ac{AG} is acceptable.
The proposed \ac{AG} does not take up too much running time, because the extraction of different prior attentions, i.e., sequence-based prior attention, syntax-based prior attention, and synonym-based prior attention, is completed in the preprocessing stage.

% The time costs for each \ac{PLM} with \ac{AG} on the MultiNlI dataset is about 4 hours because of the large data size, i.e., 443K sentence pairs.
The time costs for each \ac{PLM} with \ac{AG} on the MultiNlI dataset is about 4 hours.
The time costs for each \acp{PLM} with \ac{AG} on the MedNLI dataset is about 40 minutes.
The training time of \acp{PLM} with \ac{AG} on Cross-genre-IR is about 1 hour,  but the validation time and testing time will cost about 4 hours due to the large scales of the validation and test sets, i.e.,  500K and 517K sentence pairs respectively. 

In terms of parameters, the proposed \ac{AG} does not introduce any new parameters,  and all trainable parameters in each \ac{PLM} with \ac{AG} equal to the parameters of each \ac{PLM}.
For \ac{PLM} with \ac{AG} fine-tuning on different tasks, we select the learning rate from the set \{1e-6, 5e-5, 1e-5\} and training epochs from the the set \{5, 10, 20, 30\}.
We choose the best result of learning rate 1e-5 and training epochs 5, 20, and 5 for MultiNLI, MedNLI, and Cross-genre-IR datasets, respectively.
For the $\alpha$ and $\beta$ parameters in Eq.~\ref{losses}, we use the value from the set \{0.1, 0.01, 0.001, 0.0001, 0.0\} and choose the best result.

\section{Datasets}
\label{app:section:dataset}
% \mdr{Say how the newly collected dataset can be obtained, etc. See \url{https://aclrollingreview.org/authorchecklist} under reproducibility, third main bullet.}
% Our data is uploaded to \url{https://OpenReview.net} with the paper.
% The statistics and splits are described in \S\ref{section:dataset}.
% The language of the dataset is in English.
% For data prepossessing, we use all the data from the dataset.
% ~\todo{we use the utterances with turn number greater than or equal to two for training and evaluation, as the our focus is the dialogue responses with dialogue context, while the first turn does not contain dialogue context}.  
% In terms of the data collection process, we follow the previous research~\citep{zhang2021taxonomy}, except that the workers are asked to choose multiple choices from the labels.

The datasets used in this work are MultiNLI for natural language inference, MedNLI for natural language inference on medical domain and Cross-genre-IR for the across medical genres query. 
The MultiNLI dataset is publicly available at \url{https://cims.nyu.edu/~sbowman/multinli/}.
The MedNLI dataset is publicly available at \url{https://physionet.org/content/mednli/1.0.0/}.
The Cross-genre-IR dataset is publicly available at \url{github.com/chzuo/emnlp2020-cross-genre-IR}.

\section{Ethical Considerations}
\label{app:section:ethics}
% Ethics

% Authors are encouraged to include in the paper a statement of ethical considerations, including those related to collection and annotation of data and considerations of bias, potential for misuse or harm to vulnerable populations relating to any research results.

% We encourage authors to consult the following checklist, taken from the NAACL 2021 ethical review questions

% For papers presenting new datasets:

% Does the paper describe how intellectual property (copyright, etc) was respected in the data collection process?
The datasets used in this work are all publicly available without copyright issues.
% Does the paper describe how participants’ privacy rights were respected in the data collection process?
% Does the paper describe how crowd workers or other annotators were fairly compensated and how the compensation was determined to be fair?
% Does the paper indicate that the data collection process was subjected to any necessary review by an appropriate review board?
% The data collection process for the re-annotated \ac{MDMD} dataset follows the regulations of Twitter.
% The data is anonymized so the data can not be linked to a particular user.
% The crowd workers are fairly compensated with a minimum wage per hour (using the minimum wage from a Western European country)).
% The data collection process has been approved by the ethics committee of the authors' university.
% The data will be made available to researchers that agree to the ethical regulations of the ethics committee.
% For papers presenting new datasets AND papers presenting experiments on existing datasets:
% Does the paper describe the characteristics of the dataset in enough detail for a reader to understand which speaker populations the technology could be expected to work for?
% Do the claims in the paper match the experimental results, in terms of how far the results can be expected to generalize?
% Does the paper describe the steps taken to evaluate the quality of the dataset?
%
% Characteristics and quality control of the re-annotated dataset are described in Section~\ref{sec:results}.
The claims in the paper match the results and the proposed \ac{AG} can be applied to improve the performance of different \acp{PLM} on different downstream tasks.
This paper does not involve identity characteristics nor does it categorize people.
% the data will be anonymized and only shared to researchers that follow ethical regulations, so 
% During the annotation, we warn the crowd workers that the content may contain offensive content.
